# Supplementary material for: MathGen: Revealing the Illusion of Mathematical Competence through Text-to-Image Generation
Source: arXiv:2603.27959 source file (2026-08-15)
Supplement: Supplementary file 1 [file 6_Appendix.tex]

\newpage
\appendix

% \section{More Results}
% \label{appendix:more_experimental_results}
\section{Additional Benchmark Implementation Details}
This section describes several implementation aspects of the benchmark and evaluation pipeline that complement the discussion in the main paper.

\subsection{Verification Reliability}
To ensure the reliability of the script-based evaluation protocol, we perform a manual verification procedure on the evaluation subset used in experiments. Specifically, all problems in the \textit{testmini} subset are manually inspected to verify that the evaluation scripts correctly identify incorrect outputs. During this process, we intentionally test cases where the generated images violate the mathematical constraints (e.g., incorrect counts, wrong geometric relations, or incorrect shading). Through this manual auditing process, we confirm that the scripts in the \textit{testmini} evaluation set correctly flag all tested incorrect cases, providing confidence that the deterministic evaluation pipeline behaves as intended.
\subsection{Counting Verification}
The Counting domain requires verifying that the generated image contains exactly the number of target objects specified in the prompt. Unlike other domains that rely on geometric verification, counting requires reliable instance localization. We therefore employ a lightweight RT-DETR detector (R50-VD backbone) ~\cite{DBLP:conf/cvpr/ZhaoLXWWDLC24}implemented in the HuggingFace Transformers library to identify candidate objects, filter them by the target category, and obtain the final count. A generation is considered correct only when the detected number of instances exactly matches the required quantity.

\subsection{Script-Based Verification Pipeline}

All tasks in \dataset are verified using deterministic scripts. 
The verification pipeline consists of several stages.

\paragraph{Image preprocessing.}
The generated image is first normalized through standard preprocessing operations, including image loading and format validation, color space conversion (grayscale or HSV), and threshold-based foreground extraction.

\paragraph{Structural detection.}
Depending on the task type, the scripts apply classical computer vision techniques to recover geometric primitives from the image. These operations include contour detection, Hough line transforms, polygon detection, and circle detection. The extracted primitives correspond to structural elements such as rays, line segments, circles, and polygons.

\paragraph{Geometric verification.}
The recovered structures are then validated against the mathematical constraints specified in the prompt. Typical checks include verifying the number of rays originating from a shared vertex, detecting intersections between geometric primitives, validating the topology of Venn diagrams, and confirming the correctness of polygonal or polyhedral structures.

\paragraph{Logical constraint evaluation.}
Each problem defines a set of verification criteria describing the mathematical conditions that the generated image must satisfy. The evaluation script checks each criterion independently and aggregates the results through logical conjunction. A generation is considered correct only when all constraints are simultaneously satisfied.
\section{Hyperparameters and Decision Thresholds}
\label{app:hyperparams}

This section summarizes only the \emph{main} hyperparameters and decision thresholds that are necessary to reproduce the evaluation logic. 

\subsection{Global evaluation settings}
\label{app:hyperparams:global}

At the benchmark level, all generated images are evaluated at a default resolution of \texttt{1024\,\texttimes\,1024}. For the counting subset, we use the RT-DETR detector \texttt{PekingU/rtdetr\_r50vd} with a confidence threshold of \texttt{0.45}. A counting prediction is marked correct only under exact matching, i.e., the count tolerance is \texttt{0}.
\subsection{Angle evaluators}
\label{app:hyperparams:angle}

The angle scripts rely on foreground thresholding, radial peak detection, and Hough-based line extraction. The shared thresholds are
\begin{align}
    \texttt{ANGLE\_TOL\_DEG} &= 12.0, \\
    \texttt{MIN\_PEAK\_LEN\_RATIO} &= 0.10, \\
    \texttt{MIN\_PEAK\_SEP\_DEG} &= 10, \\
    \texttt{OPPOSITE\_TOL\_DEG} &= 10.0.
\end{align}
Radial candidates are accepted only when the smoothed response exceeds
\begin{equation}
    \tau_{\mathrm{peak}} = \max\!\left(8.0,\; 0.10\cdot \max(\mathrm{smooth})\right).
\end{equation}
For Hough-based line extraction, the detector uses threshold \texttt{60}, minimum line length
\begin{equation}
    \max\!\left(80,\; 0.12\cdot \min(H, W)\right),
\end{equation}
and maximum line gap \texttt{10}. In addition, several cases compare recovered sector values against canonical targets such as $40^\circ$, $70^\circ$, $110^\circ$, and $180^\circ$, sometimes with a slightly relaxed tolerance of the form \texttt{ANGLE\_TOL\_DEG + 8.0}.

\subsection{Fraction evaluators}
\label{app:hyperparams:fraction}

The fraction subset contains the largest number of case-specific constants. In practice, however, these scripts follow a small number of recurring patterns: (i) a target ratio with tolerance, (ii) color-based region selection, and (iii) basic morphology or shape constraints.

\paragraph{Representative ratio targets.}
Typical ratio targets include $1/7$, $1/5$, $2/9$, $4/9$, $1/2$, $3/4$, $5/8$, $7/12$, and $5/6$, with tolerances ranging from \texttt{0.015} to \texttt{0.10} depending on the case. More structured variants additionally verify rectangle aspect ratios, square area ratios, or circle radius ratios.

\paragraph{Shared thresholds.}
Across many fraction scripts, white-background validation uses threshold \texttt{240} together with a border width of
\begin{equation}
    \max\!\left(1,\; 0.08\cdot \min(H, W)\right).
\end{equation}
For foreground extraction, grayscale thresholds around \texttt{200} or \texttt{240} are common. Morphological cleanup typically uses kernels such as \texttt{(3,3)}, \texttt{(5,5)}, or \texttt{(15,15)}. Minimum contour areas are usually set around \texttt{1000} or \texttt{10000}, depending on the expected object scale. In color-specific cases, the main additional constraints are simple saturation/value thresholds and purity checks, rather than materially different decision logic.

\subsection{Set evaluators}
\label{app:hyperparams:set}

The set scripts mainly depend on Hough-circle detection and region occupancy validation. The shared circle-detection parameters are
\begin{align}
    dp &= 1.2, & \texttt{min\_dist} &= 100.0, \\
    \texttt{param1} &= 50.0, & \texttt{param2} &= 30.0, \\
    \texttt{min\_radius} &= 80.
\end{align}
Region correctness is then evaluated using red-occupancy thresholds
\begin{equation}
    \tau_{\mathrm{on}} = 0.20, \qquad \tau_{\mathrm{off}} = 0.05,
\end{equation}
meaning that a region expected to be filled must exceed $0.20$, whereas a region expected to remain empty must stay below $0.05$. Some variants use slightly stricter values, but the overall verification logic remains the same.

\subsection{Plane and solid evaluators}
\label{app:hyperparams:geometry}

The plane and solid subsets are implemented primarily through shared geometry utilities rather than heavily individualized case scripts. Consequently, the most important parameters are relative geometric thresholds tied to image size. In the plane scripts, representative values include a filled-dot Hough detector with \texttt{dp = 1.2}, \texttt{param1 = 100}, and \texttt{param2 = 12}; candidate marker radii constrained to \texttt{[0.0025, 0.014]$\cdot\min(H,W)$}; minimum marker spacing \texttt{0.03$\cdot\min(H,W)$}; and a filled-dot acceptance ratio of at least \texttt{0.68}. The main circle is further constrained by radius and border-margin checks. The solid scripts follow the same design philosophy, using shared contour-area cutoffs and relative geometric consistency thresholds for polygons, edges, and occupied regions.

\subsection{Function evaluators}
\label{app:hyperparams:function}

The function subset is more heterogeneous than the other domains, so we report only the representative numerical thresholds that characterize the common verification pipeline rather than listing case-by-case settings. Across this subset, the evaluators typically use edge detection with thresholds in the range of \texttt{50--150}, Hough-based line extraction with thresholds around \texttt{120} and maximum line gaps around \texttt{25}, and axis masking or localization with widths around \texttt{10} pixels. For asymptote or structural recovery, the scripts commonly use search windows of about \texttt{30} pixels, minimum valid run lengths of about \texttt{25}, and smoothing kernels around \texttt{41}. When OCR is involved, the minimum confidence threshold is typically around \texttt{12.0}. For geometric or functional fitting, the scripts use robust estimation with on the order of \texttt{250} RANSAC iterations, together with inlier tolerances around \texttt{0.35} in the horizontal direction and \texttt{0.75} in the vertical direction. Final verification is then based on whether the recovered curve or graph matches the target relation within a small numerical tolerance, typically around \texttt{0.6}.

\section{Additional Qualitative Examples and Verification Scripts}

\begin{figure}
    \centering
    \includegraphics[width=1\linewidth]{fig/apx/case/fraction.pdf}
    \caption{Examples on the Fraction Topic.}
    \label{fig:fraction_examples}
\end{figure}

\begin{figure}
    \centering
    \includegraphics[width=1\linewidth]{fig/apx/case/set.pdf}
    \caption{Examples on the Set Topic.}
    \label{fig:set_examples}
\end{figure}
\begin{figure}
    \centering
    \includegraphics[width=1\linewidth]{fig/apx/case/counting.pdf}
    \caption{Examples on the Counting Topic.}
    \label{fig:counting_examples}
\end{figure}
\begin{figure}
    \centering
    \includegraphics[width=1\linewidth]{fig/apx/case/angle.pdf}
    \caption{Examples on the Angle Topic.}
    \label{fig:angle_examples}
\end{figure}
\begin{figure}
    \centering
    \includegraphics[width=0.75\linewidth]{fig/apx/case/funciton.pdf}
    \caption{Examples on the Function Topic.}
    \label{fig:function_examples}
\end{figure}
\begin{figure}
    \centering
    \includegraphics[width=1\linewidth]{fig/apx/case/plane.pdf}
    \caption{Examples on the Plane Geometry Topic.}
    \label{fig:plane_examples}
\end{figure}

\begin{figure}
    \centering
    \includegraphics[width=0.9\linewidth]{fig/apx/case/solid.pdf}
    \caption{Examples on the Solid Geometry Topic.}
    \label{fig:solid_examples}
\end{figure}

\begin{figure}[t]
    \centering
    \includegraphics[width=\linewidth]{fig/apx/script/set1.pdf}
    \caption{Example script for set verification.}
    \label{fig:set_script}
\end{figure}

\begin{figure}[t]
    \centering
    \includegraphics[width=\linewidth]{fig/apx/script/set2.pdf}
    \caption{Example script for set verification.}
    \label{fig:set_script2}
\end{figure}

\begin{figure}
    \centering
    \includegraphics[width=1\linewidth]{fig/apx/script/fraction.pdf}
    \caption{Example script for fraction verification.}
    \label{fig:fraction_script1}
\end{figure}
\begin{figure}
    \centering
    \includegraphics[width=1\linewidth]{fig/apx/script/fraction1.pdf}
    \caption{Example script for fraction verification.}
    \label{fig:fraction_script2}
\end{figure}

\begin{figure}[t]
    \centering
    \includegraphics[width=\linewidth]{fig/apx/script/angle1.pdf}
    \caption{Example script for angle verification.}
    \label{fig:angle_script}
\end{figure}

\begin{figure}[t]
    \centering  
    \includegraphics[width=\linewidth]{fig/apx/script/function1.pdf}
    \caption{Example script for function verification.}
    \label{fig:function_script1}
\end{figure}

\begin{figure}[t]
    \centering
    \includegraphics[width=\linewidth]{fig/apx/script/function2.pdf}
    \caption{Example script for function verification.}
    \label{fig:function_script2}
\end{figure}

\begin{figure}[t]
    \centering
    \includegraphics[width=\linewidth]{fig/apx/script/plane1.pdf}
    \caption{Example script for plane geometry verification.}
    \label{fig:plane_script1}
\end{figure}

\begin{figure}[t]
    \centering
    \includegraphics[width=\linewidth]{fig/apx/script/plane2.pdf}
    \caption{Example script for plane geometry verification.}
    \label{fig:plane_script2}
\end{figure}

\begin{figure}[t]
    \centering
    \includegraphics[width=\linewidth]{fig/apx/script/plane3.pdf}
    \caption{Example script for plane geometry verification.}
    \label{fig:plane_script3}
\end{figure}

\begin{figure}[t]
    \centering
    \includegraphics[width=\linewidth]{fig/apx/script/solid1.pdf}
    \caption{Example script for solid geometry verification.}
    \label{fig:solid_script}
\end{figure}
\begin{figure}[t]
    \centering
    \includegraphics[width=\linewidth]{fig/apx/script/solid2.pdf}
    \caption{Example script for solid geometry verification.}
    \label{fig:solid_script2}
\end{figure}
